# Supplementary material for: Joint Constrained Learning for Event-Event Relation Extraction
Source: arXiv:2010.06727 source file (2021-05-02)
Supplement: Supplementary file 1 [file 6Appendix.tex]

\clearpage
\appendix

\section{Appendices}
\label{sec:appendix}

\subsection{RED Preprocessing}\label{sup:red}
To carry out the case study on the extended version of RED dataset, we need to do the mapping from relations in RED to relations in MATRES and HiEve, which is shown in Table 5. Other event-event relations in RED are mapped to \textsc{Vague} or \textsc{NoRel} according to their relation types, and the relations annotated between entities are disgarded.

\begin{table}[!h]
\label{tab:mapping}
\small
\centering
\begin{tabular}{l|l}
\toprule
Original labels in RED & Mapped labels\\\hline
\begin{tabular}[c]{@{}l@{}}BEFORE,\\ BEFORE/CAUSES,\\ BEFORE/PRECONDITION,\\ ENDS-ON,\\ OVERLAP/PRECONDITION\end{tabular} & \textsc{Before}                                                         \\ \hline
SIMULTANEOUS                                                                                                              & \textsc{Equal}                                                          \\ \hline
\begin{tabular}[c]{@{}l@{}}OVERLAP,\\ REINITIATES\end{tabular}                                                            & \textsc{Vague}                                                          \\ \hline
\begin{tabular}[c]{@{}l@{}}CONTAINS,\\ CONTAINS-SUBEVENT\end{tabular}                                                     & \begin{tabular}[c]{@{}l@{}}\textsc{Parent-Child} \&\\ \textsc{Before}\end{tabular} \\ \hline
BEGINS-ON                                                                                                                 & \textsc{After}                                                          \\ \bottomrule
\end{tabular}
\label{tab:RED_mapping}
\caption{Mapping from relations annotated in the RED dataset to the relations studied in this work.}
\end{table}

\subsection{More Implementation Details}
The experiments are implemented on Intel(R) Xeon(R) Gold 5218 CPU@2.30GHz, using one TITAN RTX GPU (24GB). The average runtime of the training process is about 0.4h per epoch. The total number of parameters of the model is 2401416. The table below lists the range of hyper-parameters we used in our experiments.

\begin{table}[!h]
\label{tab:hyperparam}
    \centering
    \small
    \begin{tabular}{l|l}\toprule
      Hyper-parameters & Range\\\hline
      Symmetry loss coefficient: $\lambda_S$ & [0.0, 1.0], \textbf{0.2}\\
      Conjunction loss coefficient: $\lambda_C$ & [0.0, 1.0], \textbf{0.2}\\
      
      Hidden dimension of BiLSTM & [256, 1024], \textbf{768} \\
      %Maximum token length of a sentence & 60, 90, \textbf{120}\\
      Batch size & [256, 1024], \textbf{512}\\
      Number of epochs & [40, 200], \textbf{80}\\
      Dimension of POS vectors & \textbf{18}, 35\\
      \bottomrule
    \end{tabular}
    \caption{The range of hyper-parameters considered. Bold numbers denote the hyper-parameters used to generate results. For instance, [0.0, 1.0] is the range that $\lambda_S$ can be drawn from, and 0.2 is the value that achieves the best performance. While the POS (Part-Of-Speech) tags have 35 different labels, we collapse some of the closely-related labels into one (e.g. we collapse VB, VBD, VBZ, VBP, VBN into VB) and get 18 labels.}
\end{table}

\iffalse

\subsection{Dataset Statistics}
\label{sec:datasetstat}
We briefly summarize the data statistics for HiEve, MATRES, and RED dataset in Table~\ref{tbl:stats}. In the training process, we use the training splits of HiEve and MATRES. For validation, we choose the model with best $F_1$ score on the development set of MATRES by uniformly selecting hyperparameters from the range as specified in Table 6. All of the test sets are used for reporting results.
\begin{table}[!h]
\label{tab:stat}
    \centering
    \small
    \begin{tabular}{c|c|c|c}\toprule
         & HiEve & MATRES & RED\\\hline
         \multicolumn{4}{c}{\# of Documents}\\\hline
         Train & 80 & 183 & - \\
         Dev & - & 72 & - \\
         Test & 20 & 20 & 35\\
         \midrule
          \multicolumn{4}{c}{\# of Pairs}\\
          \midrule
       Train  & 35001 & 6332 & - \\
       Test  & 7093 & 827 & 1718\\% 1032
       \bottomrule
    \end{tabular}
    \caption{Data statistics of HiEve, MATRES, and RED.}\label{tbl:stats}
    
\end{table}

\fi

\iffalse
\subsection{\textsc{NoRel} Prediction on HiEve}
\label{sec:APPEN_NOREL}
\begin{table}[]
    \centering
    \begin{tabular}{c|c}
       \textsc{TacoLM} \cite{ZNKR20}  & 91.3 \\
       StructLR \cite{glavas-etal-2014-hieve}  & \\
       \CC{20}Joint Constrained Learning (ours) & \CC{20} 90.5
    \end{tabular}
    \caption{Caption}
    \label{tab:my_label}
\end{table}
\fi
